# Supplementary material for: Failure Analysis of Big Cloud Service Providers Prior to and During Covid-19 Period
Source: arXiv:2210.08006 source file (2023-01-17)
Supplement: Supplementary file 1 [file appendix.tex]

% this file is called up by thesis.tex
% content in this file will be fed into the main document

%: ----------------------- paths to graphics ------------------------

% change according to folder and file names
\ifpdf
    \graphicspath{{10_appendix/figures/PNG/}{10_appendix/figures/PDF/}{10_appendix/figures/}}
\else
    \graphicspath{{10_appendix/figures/EPS/}{10_appendix/figures/}}
\fi

%: ----------------------- contents from here ------------------------

\chapter{Reproducibility}
\section{Abstract}

{\em Obligatory}

\section{Artifact check-list (meta-information)}

{\em Obligatory. Use just a few informal keywords in all fields applicable to your artifacts
and remove the rest. This information is needed to find appropriate reviewers and gradually 
unify artifact meta information in Digital Libraries.}

{\small
\begin{itemize}
  \item {\bf Algorithm: }
  \item {\bf Program: }
  \item {\bf Compilation: }
  \item {\bf Transformations: }
  \item {\bf Binary: }
  \item {\bf Model: }
  \item {\bf Data set: }
  \item {\bf Run-time environment: }
  \item {\bf Hardware: }
  \item {\bf Run-time state: }
  \item {\bf Execution: }
  \item {\bf Metrics: }
  \item {\bf Output: }
  \item {\bf Experiments: }
  \item {\bf How much disk space required (approximately)?: }
  \item {\bf How much time is needed to prepare workflow (approximately)?: }
  \item {\bf How much time is needed to complete experiments (approximately)?: }
  \item {\bf Publicly available?: }
  \item {\bf Code licenses (if publicly available)?: }
  \item {\bf Data licenses (if publicly available)?: }
  \item {\bf Workflow framework used?: }
  \item {\bf Archived (provide DOI)?: }
\end{itemize}
}

%%%%%%%%%%%%%%%%%%%%%%%%%%%%%%%%%%%%%%%%%%%%%%%%%%%%%%%%%%%%%%%%%%%%%
\section{Description}

\subsection{How to access}

{\em Obligatory}

\subsection{Hardware dependencies}

\subsection{Software dependencies}

\subsection{Data sets}

\subsection{Models}

%%%%%%%%%%%%%%%%%%%%%%%%%%%%%%%%%%%%%%%%%%%%%%%%%%%%%%%%%%%%%%%%%%%%%
\section{Installation}

{\em Obligatory}

%%%%%%%%%%%%%%%%%%%%%%%%%%%%%%%%%%%%%%%%%%%%%%%%%%%%%%%%%%%%%%%%%%%%%
\section{Experiment workflow}

%%%%%%%%%%%%%%%%%%%%%%%%%%%%%%%%%%%%%%%%%%%%%%%%%%%%%%%%%%%%%%%%%%%%%
\section{Evaluation and expected results}

{\em Obligatory}

%%%%%%%%%%%%%%%%%%%%%%%%%%%%%%%%%%%%%%%%%%%%%%%%%%%%%%%%%%%%%%%%%%%%%
\section{Experiment customization}

%%%%%%%%%%%%%%%%%%%%%%%%%%%%%%%%%%%%%%%%%%%%%%%%%%%%%%%%%%%%%%%%%%%%%
\section{Notes}

%%%%%%%%%%%%%%%%%%%%%%%%%%%%%%%%%%%%%%%%%%%%%%%%%%%%%%%%%%%%%%%%%%%%%
\section{Methodology}

Submission, reviewing and badging methodology:

\begin{itemize}
  \item \url{https://www.acm.org/publications/policies/artifact-review-badging}
  \item \url{http://cTuning.org/ae/submission-20201122.html}
  \item \url{http://cTuning.org/ae/reviewing-20201122.html}
\end{itemize}

\dots

\newpage
\chapter{Self Reflection}
\dots

\newpage
\chapter{Additional Experiments}
\dots

% ---------------------------------------------------------------------------
%: ----------------------- end of thesis sub-document ------------------------
% ---------------------------------------------------------------------------
